# Supplementary material for: Rethinking Few-shot 3D Point Cloud Semantic Segmentation
Source: arXiv:2403.00592 source file (2024-03-01)
Supplement: Supplementary file 1 [file X_suppl.tex]

\clearpage
\setcounter{page}{1}
\maketitlesupplementary

\section{More details about the original biased sampling}
\label{sec:rationale}
\begin{algorithm}
\caption{The original biased sampling method}\label{alg:smp}
\KwData{point cloud $\{P_1,..,P_N\}$, sampling number $M$, foreground class $C$, valid points $VP$, foreground sampling number $FG$}
\KwResult{sampled point cloud $\{P_{i_1},..,P_{i_M}\}$}
$VP \gets \{P_i~|~labelof(P_i) = C\}$\;
  \eIf{$N < P$}{
    $FG \gets sizeof(VP)$\;
  }{
    $FG \gets P \times \frac{VP}{N}$\;
    }
$PC_1 \gets$ sample $FG$ points from $VP$\;
$PC_2 \gets$ sample $P - FG$ points from $\{P_1,..,P_N\}$\;
$\{P_{i_1},..,P_{i_M}\} = PC_1 \cup PC_2$\;
\end{algorithm}

Having the supplementary compiled together with the main paper means that:
\begin{itemize}
\item The supplementary can back-reference sections of the main paper, for example, we can refer to \cref{sec:intro};
\item The main paper can forward reference sub-sections within the supplementary explicitly (e.g. referring to a particular experiment); 
\item When submitted to arXiv, the supplementary will already included at the end of the paper.
\end{itemize}
To split the supplementary pages from the main paper, you can use \href{https://support.apple.com/en-ca/guide/preview/prvw11793/mac#:~:text=Delete%20a%20page%20from%20a,or%20choose%20Edit%20%3E%20Delete).}{Preview (on macOS)}, \href{https://www.adobe.com/acrobat/how-to/delete-pages-from-pdf.html#:~:text=Choose%20%E2%80%9CTools%E2%80%9D%20%3E%20%E2%80%9COrganize,or%20pages%20from%20the%20file.}{Adobe Acrobat} (on all OSs), as well as \href{https://superuser.com/questions/517986/is-it-possible-to-delete-some-pages-of-a-pdf-document}{command line tools}.
